# Supplementary material for: Non-adiabatic Kohn Anomaly in Heavily Boron-doped Diamond
Source: arXiv:1706.02151 source file (2017-06-07)
Supplement: Supplementary file 1 [file supplemental.pdf]

# Supplemental Material for
# 'Non-adiabatic Kohn Anomaly in Heavily Boron-doped Diamond'

Fabio Caruso,[1] Moritz Hoesch,[2] Philipp Achatz,[3] Jorge Serrano,[4]
Michael Krisch,[5] Etienne Bustarret,[3] and Feliciano Giustino[1]

[1] *Department of Materials, University of Oxford, Parks Road, Oxford, OX1 3PH, United Kingdom*
[2] *Diamond Light Source, Harwell Campus, Didcot OX11 0DE, United Kingdom*
[3] *Univ. Grenoble Alpes, CNRS, Inst. NEEL, F-38000 Grenoble, France*
[4] *Yachay Tech University, School of Physical Sciences and Nanotechnology, 100119-Urcuquí, Ecuador*
[5] *European Synchrotron Radiation Facility, 6 rue Jules Horowitz, 38043 Grenoble Cedex, France*

Supplemental Table I. Coordinates of the scattering vectors **Q** of the IXS spectra in units of $2\pi/a$, with $a = 3.67$ Å.

| Index | $Q_x$ | $Q_y$ | $Q_z$ |
|---|---|---|---|
| 1 | 2.06 | 0.00 | 0.00 |
| 2 | 2.18 | −0.03 | 0.00 |
| 3 | 2.29 | −0.06 | 0.00 |
| 4 | 2.41 | −0.09 | 0.00 |
| 5 | 2.52 | −0.13 | 0.00 |
| 6 | 2.56 | 0.00 | 0.00 |
| 7 | 2.67 | −0.03 | 0.00 |
| 8 | 2.78 | −0.06 | 0.00 |
| 9 | 2.89 | −0.08 | 0.00 |
| 10 | 3.00 | −0.12 | 0.00 |

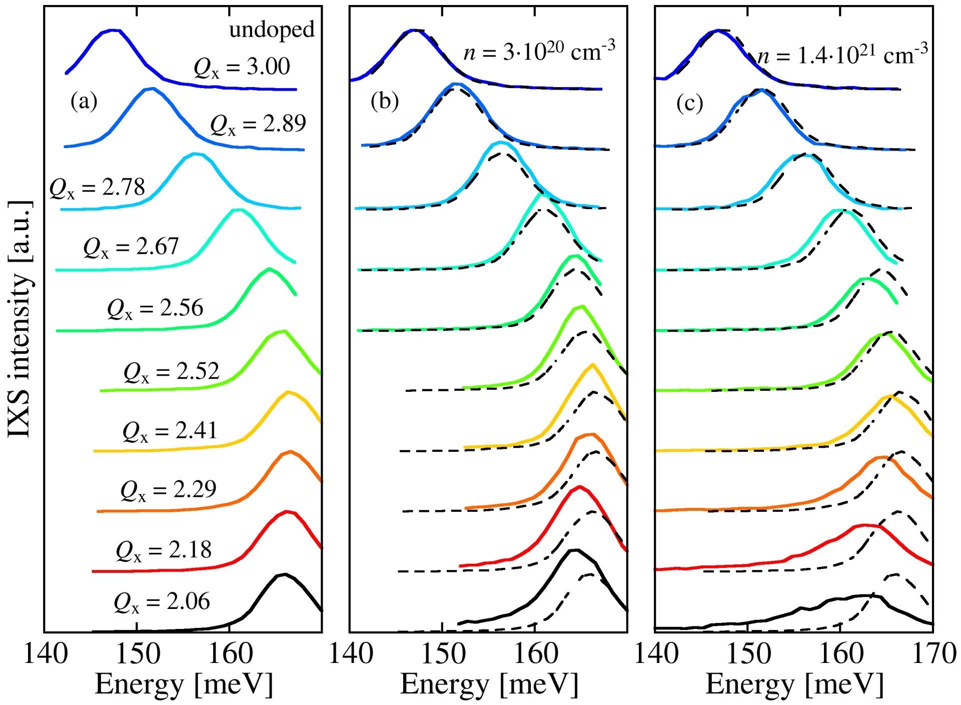


Supplemental Figure 1. Inelastic x-ray scattering (IXS) spectra for scattering vectors **Q** varied from (2.06,0,0) to (3,−0.12,0) in units of $2\pi/a$, with $a = 3.67$ Å. (a) pristine diamond, (b) B-doped diamond with $n = 3 \cdot 10^{20}$ cm$^{-3}$ and (c) $1.4 \cdot 10^{21}$ cm$^{-3}$. The IXS spectra of the undoped sample are reported as dashed lines in (b) and (c) for comparison. The IXS spectral intensity has been rescaled by the maximum intensity of the phonon peak for **Q** =(3,−0.12,0).

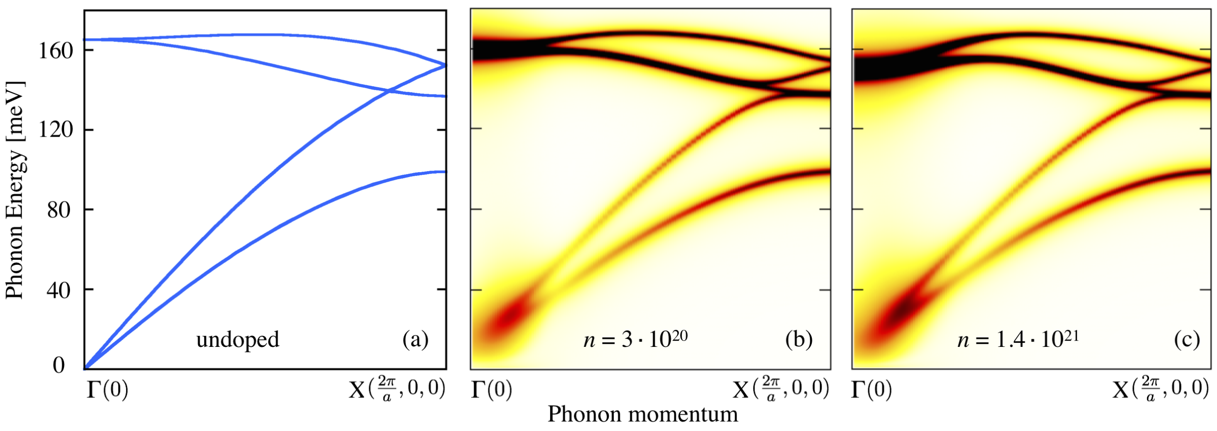


Supplemental Figure 2. (a) Phonon dispersions of pristine diamond as obtained from density functional perturbation theory. (b)-(c) Full non-adiabatic spectral function of diamond for B-doping concentrations of $n = 3 \cdot 10^{20}$ cm$^{-3}$ and $n = 1.4 \cdot 10^{21}$ cm$^{-3}$.

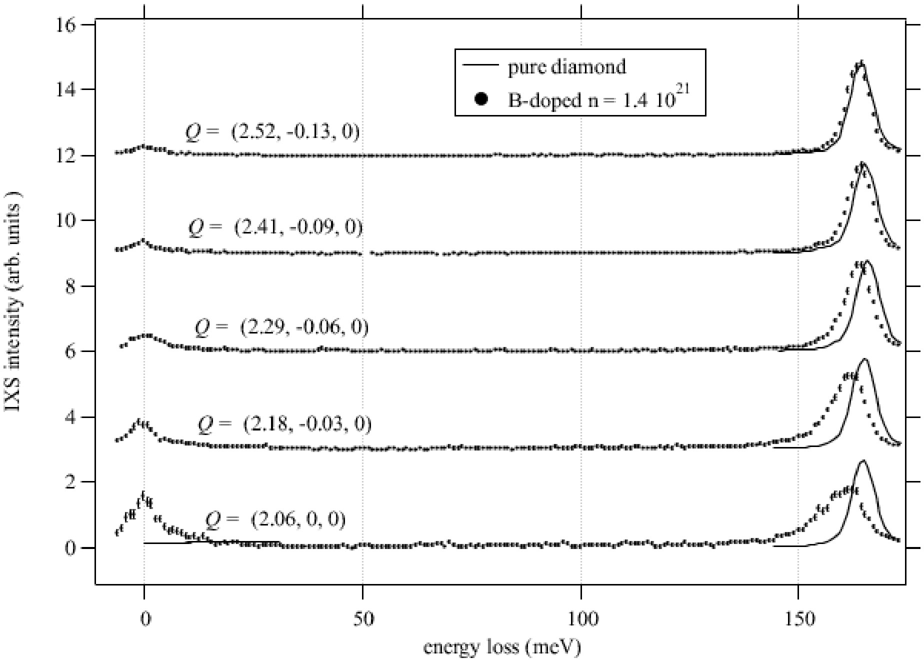


Supplemental Figure 3. Inelastic x-ray scattering (IXS) spectra in the full spectral range for scattering vectors $\mathbf{Q}$ varied from (2.06,0,0) to (2.52,−0.13,0) in units of $2\pi/a$, with $a = 3.67$ Å for pristine diamond (straight line) and B-doped diamond with $n = 1.4 \cdot 10^{21}$ cm$^{-3}$ (dots).

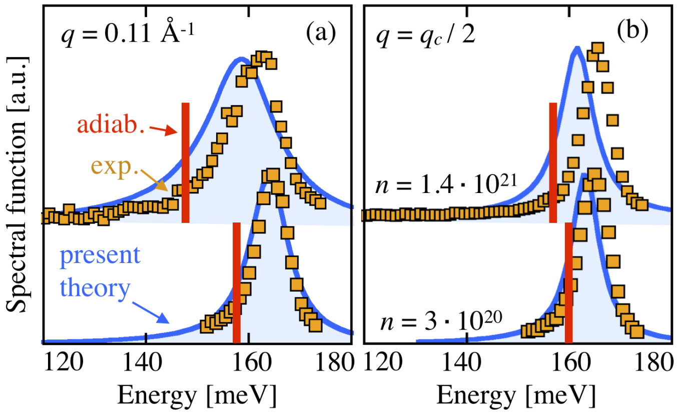


Supplemental Figure 4. Phonon lineshapes for doping concentrations of $1.4 \cdot 10^{21}$ cm$^{-3}$ (top) and $3 \cdot 10^{20}$ cm$^{-3}$ (bottom) for momentum transfers of (a) $q = 0.11$ Å$^{-1}$, and (b) $q = q_c/2$ along the Γ-X direction.Due to the infinitesimal linewidths, the adiabatic peaks are represented as vertical lines.
